# Supplementary material for: 3D Equivariant Pose Regression via Direct Wigner-D Harmonics Prediction
Source: arXiv:2411.00543 source file (2024-11-04)
Supplement: Supplementary file 1 [file supp_0_preliminary.tex]

\section{Spherical Harmonics \& Wigner-D Matrix}\label{sec:supp_spherical_harmonics_and_wigner_d}

We explain a detailed derivation of 3D rotation in harmonics domain. We first define spherical harmonics and explain the   Wigner-D matrix transformation.

\subsection{Spherical harmonics}
Spherical harmonics are a set of mathematical functions that serve as a basis for representing functions on the surface of a sphere. In the context of \(\text{SO}(3)\) pose estimation, they are instrumental for representing and processing orientations in three-dimensional space. Specifically, spherical harmonics are defined by the equation 
\begin{equation}
Y_l^m(\theta, \phi) = \sqrt{\frac{(2l+1)(l-m)!}{4\pi (l+m)!}} P_l^m(\cos \theta) e^{im\phi}    
\end{equation}
where \(l\) and \(m\) are the degree and order of the harmonic, \(\theta\) and \(\phi\) are the polar and azimuthal angles, respectively, \(P_l^m\) are the associated Legendre polynomials, and \(e^{im\phi}\) is the complex exponential. In \(\text{SO}(3)\) pose estimation, these functions allow for the efficient representation and manipulation of rotational data, facilitating tasks like rotation-invariant object recognition and orientation filtering in 3D space.

\subsection{Wigner-D Matrix }

The Wigner-D matrix, denoted as \(D^l_{m,n}(\alpha, \beta, \gamma)\), is a unitary matrix used to describe rotations in three-dimensional space and is particularly valuable in pose estimation applications. It represents elements of the rotation group SO(3), which is essential for modeling the orientation of objects in 3D space. The matrix is characterized by the angular momentum quantum number \(l\) and the magnetic quantum numbers \(m\) and \(n\), ranging from \(-l\) to \(l\).  The Euler angles \(\alpha\), \(\beta\), and \(\gamma\) define the rotation around the z-axis, the new y-axis, and the new z-axis, respectively. The matrix is given by:
\begin{equation}
D^l_{m,n}(\alpha, \beta, \gamma) = e^{-i m \alpha} d^l_{m,n}(\beta) e^{-i n \gamma}    ,
\end{equation}
where \(d^l_{m,n}(\beta)\) is the real-valued Wigner small-d matrix.
In the context of pose estimation, the Wigner-D matrix provides a robust framework for modeling 3D rotations of objects detected in images. This matrix allows for the precise transformation and comparison of different poses by providing a complete and compact representation of rotations.

The Wigner-D matrices are also closely related to spherical harmonics, which are often used in pose estimation for representing and analyzing angular functions on a sphere. The angular momentum quantum number \(l\) in the Wigner-D matrix corresponds to the degree of the spherical harmonic, indicating the frequency level or the number of oscillations on the sphere. The magnetic quantum numbers \(m\) and \(n\) correspond to the order of the spherical harmonic, representing variations in the azimuthal direction. Spherical harmonics can be rotated using the Wigner-D matrices, facilitating the manipulation of spherical functions under rotations. Specifically, a spherical harmonic \(Y_l^m(\theta, \phi)\) under rotation transforms according to:
\begin{equation}
Y_l^n(\theta', \phi') = \sum_{m=-l}^{l} D^l_{m,n}(\alpha, \beta, \gamma) Y_l^{m}(\theta, \phi),    
\end{equation}
Here, \(\alpha\), \(\beta\), and \(\gamma\) are the Euler angles defining the rotation, and \(D^l_{m,n}(\alpha, \beta, \gamma)\) are the components of the Wigner-D matrix for a given quantum number \(l\).

This relationship illustrates how Wigner-D matrices serve as rotational operators for spherical harmonics, thus enabling accurate and efficient pose estimation by transforming spherical functions in a mathematically consistent manner. This capability is critical in fields such as computer vision, robotics, and augmented reality, where understanding and manipulating the orientation of objects in 3D space is essential. The application of Wigner-D matrices in these areas enhances the accuracy and robustness of pose estimation algorithms, making them an indispensable tool in modern computational analysis.

\subsubsection{Definition of Euler Angles}
The Euler angles $(\alpha, \beta, \gamma)$ define a rotation in three dimensions, typically decomposed into three successive rotations:
\[
R(\alpha, \beta, \gamma) = R_z(\gamma) R_y(\beta) R_z(\alpha)
\]
where $R_z(\theta)$ and $R_y(\theta)$ are rotations about the z-axis and y-axis respectively, defined as:
\[
R_z(\theta) = \begin{bmatrix}
\cos \theta & -\sin \theta & 0 \\
\sin \theta & \cos \theta & 0 \\
0 & 0 & 1
\end{bmatrix}, \quad
R_y(\theta) = \begin{bmatrix}
\cos \theta & 0 & \sin \theta \\
0 & 1 & 0 \\
-\sin \theta & 0 & \cos \theta
\end{bmatrix}
\]

\subsubsection{Detailed Expression for Wigner $D$ Matrix}\label{sec:detailed_wigner_d}
The Wigner $D$ matrix elements for quantum mechanical rotations in angular momentum eigenstates are given by
$ D^l_{m,n}(\alpha, \beta, \gamma) = e^{-i m \gamma} d^l_{m,n}(\beta) e^{-i n \alpha}$.
Here, $d^l_{m,n}(\beta)$ is the small Wigner $D$ matrix, described by:
\begin{equation}
d^l_{m,n}(\beta) = \sum_k \frac{(-1)^k \sqrt{(l+m)!(l-m)!(l+n)!(l-n)!}}{(l-m-k)!(l+n-k)!k!(k+m-n)!} \left( \cos \frac{\beta}{2} \right)^{2l-2k+n-m} \left( \sin \frac{\beta}{2} \right)^{2k+m-n}
\end{equation}
The sum over $k$ is constrained such that all factorial arguments remain non-negative.
